# Supplementary material for: On the Necessity and Effectiveness of Learning the Prior of Variational Auto-Encoder
Source: arXiv:1905.13452 source file (2019-05-31)
Supplement: Supplementary file 1 [file gaussian_px_given_z_extrema.tex]

\begin{proposition*}
	For finite number of discrete training data, \ie{}, the training distribution $p^{\star}(\vv{x}) = \frac{1}{N} \sum_{i=1}^N \delta(\vv{x}-\vv{x}^{(i)})$, if we let $p_{\theta}(\vv{x}|\vv{z}) = \mathcal{N}(\vv{\mu}_{\theta}(\vv{z}),\sigma^2 \vv{I})$, where $\vv{\mu}_{\theta}(\vv{z})$ is produced by the decoder and $\sigma$ is a global fixed constant, then for any particular encoder $q_{\phi}(\vv{z}|\vv{x})$ and prior $p_{\lambda}(\vv{z})$, the optimal decoder $\vv{\mu}_{\theta}(\vv{z})$ is:
	\begin{equation*}
		\vv{\mu}_{\theta}(\vv{z}) = \sum_i w_i(\vv{z})\,\vv{x}^{(i)}, \quad \text{where} \;\,
		w_i(\vv{z}) = \frac{q_{\phi}(\vv{z}|\vv{x}^{(i)})}{\sum_j q_{\phi}(\vv{z}|\vv{x}^{(j)})} \;\, \text{and}\;\, \sum_i w_i(\vv{z}) = 1
	\end{equation*}
\end{proposition*}

\begin{proof}
	The training objective $\mathcal{L}$ can be formulated as:
	\begin{align*}
		\mathcal{L} &= \E_{p^{\star}(\vv{x})}\,\E_{q_{\phi}(\vv{z}|\vv{x})}\left[\log p_{\theta}(\vv{x}|\vv{z}) + \log \frac{p_{\theta}(\vv{z})}{q_{\phi}(\vv{z}|\vv{x})} \right] \\
		&= \iint p^{\star}(\vv{x}) \, q_{\phi}(\vv{z}|\vv{x}) \left(\log p_{\theta}(\vv{x}|\vv{z}) + \log \frac{p_{\theta}(\vv{z})}{q_{\phi}(\vv{z}|\vv{x})} \right) \dd{\vv{z}} \, \dd{\vv{x}} \\
		&= \iint p^{\star}(\vv{x}) \, q_{\phi}(\vv{z}|\vv{x}) \left[ \sum_k \left( -\frac{\left(x_k - \mu_{\theta}^k(\vv{z})\right)^2}{2\sigma^2} - \log \sqrt{2\pi}\sigma \right) + \log \frac{p_{\theta}(\vv{z})}{q_{\phi}(\vv{z}|\vv{x})} \right] \dd{\vv{x}} \, \dd{\vv{z}} \\
		&= \int F(\vv{z},\vv{\mu}_{\theta}) \,\dd{\vv{z}}
	\end{align*}
	where $x_k$ is the $k$-th dimension of $\vv{x}$, $\mu^{k}_{\theta}(\vv{z})$ is the $k$-th dimension of $\vv{\mu}_{\theta}(\vv{z})$, and $F(\vv{z},\vv{\mu}_{\theta})$ is:
	\begin{equation*}
		F(\vv{z},\vv{\mu}_{\theta}) = \int p^{\star}(\vv{x}) \, q_{\phi}(\vv{z}|\vv{x}) \left[ \sum_k \left( -\frac{\left(x_k - \mu_{\theta}^k(\vv{z})\right)^2}{2\sigma^2} - \log \sqrt{2\pi}\sigma \right) + \log \frac{p_{\theta}(\vv{z})}{q_{\phi}(\vv{z}|\vv{x})} \right] \dd{\vv{x}}
	\end{equation*}
	According to Euler's equation~\citep[page 14 and 35]{gelfandCalculusVariations2000}, the necessary condition for $\mathcal{L}$ to have an extremum for a given $\vv{\mu}_{\theta}$ is that, $\vv{\mu}_{\theta}(\vv{z})$ satisfies $\partial F / \partial \mu_{\theta}^k = 0, \forall k$.  Thus we have:
	\begin{align*}
		 \frac{\partial F}{\partial \mu_{\theta}^k} = 0 
		\implies & \int p^{\star}(\vv{x}) \, q_{\phi}(\vv{z}|\vv{x}) \left[-\frac{x_k - \mu_{\theta}^k(\vv{z})}{2\sigma^2}\cdot 2 \cdot (-1)\right] \,\dd{\vv{x}} = 0 \\
		\implies & \int p^{\star}(\vv{x}) q_{\phi}(\vv{z}|\vv{x}) \left[x_k - \mu_{\theta}^k(\vv{z})\right] \,\dd{\vv{x}} = 0 \\
		\implies & \sum_i q_{\phi}(\vv{z}|\vv{x}^{(i)})\left[x_k^{(i)} - \mu^k_{\theta}(\vv{z})\right] = 0 \\
		\implies & \sum_i q_{\phi}(\vv{z}|\vv{x}^{(i)}) \, x_k^{(i)} = \left(\sum_i q_{\phi}(\vv{z}|\vv{x}^{(i)})\right) \mu_{\theta}^k(\vv{z}) \\
		\implies & \mu_{\theta}^k(\vv{z}) = \frac{\sum_i q_{\phi}(\vv{z}|\vv{x}^{(i)})\,x_k^{(i)}}{\sum_j q_{\phi}(\vv{z}|\vv{x}^{(j)})}
	\end{align*}
	That is to say, $\vv{\mu}_{\theta}(\vv{z}) = \frac{\sum_i q_{\phi}(\vv{z}|\vv{x}^{(i)})\,\vv{x}^{(i)}}{\sum_j q_{\phi}(\vv{z}|\vv{x}^{(j)})} = \sum_i w_i(\vv{z})\,\vv{x}^{(i)}$.
\end{proof}
